# Supplementary material for: Multi-Level Fine-Tuning, Data Augmentation, and Few-Shot Learning for Specialized Cyber Threat Intelligence
Source: arXiv:2207.11076 source file (2022-07-22)
Supplement: Supplementary file 1 [file appendix.tex]

\section*{Appendices} \label{appendix}
\addcontentsline{toc}{section}{Appendices}

\setcounter{subsection}{0}

\subsection{Availability of Data and Material} \label{appendix_data_material}
In summary, most datasets analyzed during the current study are publicly available. In the \textbf{first evaluation} (section \ref{results_1}), we used the SST dataset\footnote{SST datasets of \citet{Socher2013}: \url{https://nlp.stanford.edu/sentiment/index.html}} of \citet{Socher2013} which is publicly available.

The datasets analyzed during the \textbf{second evaluation} (section \ref{results_2}) are not publicly available due to publication restrictions by news agencies. Still, a concise description of these datasets is given in appendix \ref{appendix_dataset}. We would like to highlight that news classification is a highly relevant field in the industry that receives too little attention in academia. In addition, we had to decide to create our own dataset in order to tackle long text classification, as these datasets are particularly rare.  We hope that we have included enough results from the public datasets so that reproducibility can be inferred.

For the \textbf{third evaluation} (section \ref{results_3}), three public datasets (Boston Bombings, the Bohol Earthquake and the West Texas Explosions) from the CrisisLexT26 \footnote{CrisisLexT26 datasets from \citet{Olteanu2015}: \url{https://github.com/sajao/CrisisLex/tree/master/data/CrisisLexT26}} annotated data groups from \citet{Olteanu2015} and two public datasets (Dublin and New York City) from the annotated data groups from \citet{Schulz2017}\footnote{Datasets from \citet{Schulz2017}: \url{ http://www.doc.gold.ac.uk/~cguck001/IncidentTweets/}}  were used. The primary language of all datasets is English.

%Most of the data analyzed during this study are openly available:
%\begin{itemize}
%    \item \citep{Socher2013}: \url{https://nlp.stanford.edu/sentiment/index.html}
%    \item \citep{Olteanu2015}: \url{https://github.com/sajao/CrisisLex/tree/master/data/CrisisLexT26}
%    \item \citep{Schulz2017} \url{http://www.doc.gold.ac.uk/~cguck001/IncidentTweets/}
%\end{itemize}
%Some of the data analyzed in the current study is not publicly available due to publication restrictions by news agencies. However, we would like to highlight that news classification is a highly relevant field in the industry that receives too little attention in academia. In addition, we had to decide to create our own dataset in order to tackle long text classification, as these datasets are particularly rare. We hope that we have included enough results from the public datasets so that reproducibility can be inferred.

\subsection{Description of the Datasets Used During the Second Evaluation} \label{appendix_dataset}
The datasets consist of English news articles of over 2,600 different source domains from the years 2019 and 2020, which were preselected with regard to specific query words. For each topic, the articles received values on the basis of these query words to split them into 12 different buckets. We sampled the news articles from these buckets uniformly so that highly diverse instances were labeled. A short summary of the labeling guidelines and data distributions are described in the following list:

\textbf{Layoff.} The layoff topic consists of all forms of dismissals of employees in the corporate context. A total of 1992 articles were annotated of which 751 instances are positive and 1241 are negative.

\textbf{Management change.} This topic covers all forms of changes (retirement, resignation, appointment) of the board of directors and important positions in companies, organizations and advisory boards. 2129 instances were labeled of which 567 instances are positive and 1562 are negative.

\textbf{Mergers and Acquisitions.} M\&A includes all transactions in which ownership is transferred to companies or their operating units. The mere investment in a company is seen as negative here. For this topic, 2227 instances were labeled of which 474 are positive and 1753 are negative.

\textbf{Flood.} The flooding topic is positively recognized in news if the article deals with the actual flooding or the main topic is a consequence of a flood. If only an increase in the water level is reported, this message should not be regarded as positive. There are 2533 identified instances on this topic, 1639 of which are positive and 894 are negative. Although more positive than negative instances were identified here, the negative class is still seen as the majority class since the clear majority of all messages on the Internet are not related to floods. 

\textbf{Wildfire.} All forms of wildfire are classified under this topic. House fires and metaphorical uses of the term are labeled negatively. The dataset includes 2410 identified instances of which 1202 are positive and 1208 are negative. Similar to the flood topic, the negative class is the majority class.

In the preprocessing step we added the tokens “xxtitle” before every title and “xxbodytext” before the start of the normal article text.

\subsection{Algorithm} \label{appendix_algorithm}
In the following, we defined the algorithm of the context independent data augmentation method.

\begin{algorithm}
\SetAlgoLined
\SetKwInOut{Input}{Input}
\Input{Language Model $LM$, Class data $X_c$,\\ Document Embedding Model $E$,\\ Number of instances per training data $n$}
1. For each instance in $X_c$: Attach `$<|startoftext|> |i|$' to the beginning and `$<|endoftext|>$' to the end of the $i$th instance to obtain $X_{cprep}$\\
2. Finetune $LM$ on $X_{cprep}$ to obtain $LM_{cprep}$\\
3. For each k in $|X_{cprep}|$: Generate $n$ new instances with $LM_{cprep}$  and `$<|startoftext|> |i|$' as prefix to obtain $X_{gen}$\\
4. Embed all instances in $X_{gen}$ and $X_{c}$ with $E$ \\
5. Obtain $X_{filtered}$ by including all instances of $X_{gen}$ at which the embedding representations are close to the centroid of the embedded $X_{c}$

\KwResult{$X_{filtered}$ }
 \caption{Augmentation of Short Texts}
\end{algorithm}

\begin{algorithm}
\SetAlgoLined
\SetKwInOut{Input}{Input}
\Input{Language Model $LM$, Class data $X_c$,\\ Document Embedding Model $E$,\\ Number of instances per training data $n$, \\ Function extracting context part $cont()$}
1. For each instance in $X_c$: Attach `$<|startoftext|>$' to the beginning and `$<|endoftext|>$' to the end of the instances to obtain $X_{cprep}$\\
2. Finetune $LM$ on $X_{cprep}$ to obtain $LM_{cprep}$\\
3. For each $t$ in $X_{cprep}$: Generate $n$ new instances with $LM_{cprep}$  and `$<|startoftext|>$' + $cont(t)$ as prefix to obtain $X_{gen}$\\
4. Embed all instances in $X_{gen}$ and $X_{c}$ with $E$ \\
5. Obtain $X_{filtered}$ by including all instances of $X_{gen}$ at which the embedding representations are close to the centroid of the embedded $X_{c}$

\KwResult{$X_{filtered}$ }
 \caption{Augmentation of Long Texts}
 
\end{algorithm}
\subsection{Ethics} \label{appendix_ethics}
In our work, we have placed particular emphasis on ethics and repeatedly reassessed our approach with regard to responsibilities. We have restricted ourselves to only using the textual content and the labels in the datasets to respect privacy as much as possible. When working with social media data, we especially did not use, aggregate or draw any conclusion from further metadata such as the name or location of a user. 

For the practical implementation of our method, we want to mention that the GPT-2 model as well as most other language models contain biases (for example a gender, religious or racial bias) \citep{Solaiman2019}. Using the method in a real application can result in a domain shift and/or an inclusion of those biases. This can explicitly lead to discriminatory decisions by the machine learning model, even if the dataset itself does not contain any bias.

\subsection{Architecture, Hyperparameters and Infrastructure} \label{appendix_architecture}
In the evaluation, we used the pre-trained ULMFit model by \citet{Howard2018} as implemented in fastai \citep{Howard2020}. The model consists of a pre-trained encoder that is based on the AWD-LSTM architecture by \citet{Merity2018} and a linear pooling classifier. The classifier consists of a layer that concatenates the final outputs of the encoder with the maximum and the average of all intermediate outputs and two fully connected layers\footnote{ULMFit implementation: \url{https://fastai1.fast.ai/text.learner.html\#text_classifier_learner}}. Further information about the general architecture can be extracted from the paper of \citet{Howard2018} and the implementation in fastai \citep{Howard2020}. 
The encoder finetuning is done by preparing all available data of the respective task (including the augmented data) for the language modeling task. In the training, we performed 15 cycles with the 1cycle policy by \citet{Smith2018}. We used a learning rate of 0.002 and a maximum and minimum momentum of 0.8 and 0.7. Overall, we used a fixed batch size of 64 and a backpropagation through time window of 70. Each encoder and classifier was trained to the downstream task with three cycles with gradual unfreezing and another five cycles with the unfrozen model. The learning rate was individually determined by the learning rate range test by \citet{Smith2018} with a range from $10^{-7}$ to 10 over 100 iterations\footnote{Learning rate range test implementation: \url{https://fastai1.fast.ai/callbacks.lr_finder.html\#callbacks.lr_finder}}. On the outputs we used label smoothing with an epsilon parameter of 0.1. As optimization algorithm, we used the Adam algorithm \citep{Kingma2015}.

For the text generation, we used the gpt-2-simple implementation\footnote{gpt-2-simple implementation:
\url{https://github.com/minimaxir/gpt-2-simple}}  to finetune and generate texts from the GPT-2 model. Only the parameters discussed in chapter 4.2 were varied. For the filtering step, Sentence-BERT\footnote{Sentence-BERT implementation: \url{https://github.com/UKPLab/sentence-transformers}}  \citep{Reimers2019} with the “roberta-large-nli-stsb-mean-tokens” transformer model was used.

We tokenized all datasets with the built-in tokenizers of the gpt-2-simple, Sentence-BERT and fastai libraries for the different use cases.

The evaluation of chapter 4.4 was performed on a Nvidia Quadro RTX 6000 graphics card with 24 GB RAM. For the evaluation of chapter 4.3 and 4.5, less resources were necessary, which is why a Nvidia Tesla P100 with 16GB RAM was used.

In general, the tasks were quite resource intensive. The finetuning of the GPT-2 model on the flood dataset took about five hours, while the generation of ten examples per instance occupied about four days. The finetuning of the language model and the training of the classifier together took about another four hours.

\subsection{Generated Data} \label{appendix_data}

\begin{table*}[t]
\centering
\caption{Generated data instances and their most similar original counterparts.}
\label{table:generated_data}
\begin{tabularx}{\textwidth}{lX}
\hline
\multirow{10}{*}{\begin{tabular}[c]{@{}c@{}}West Texas \\ Explosions\end{tabular}} &
  Media Matters Texas:  West, Texas, fertilizer plant: 28 years, no full inspection: Before 270 tons of ammonium nitratet exploded at ... http://t.co/XwUwgRcGDT \\
 &
  West, Texas, fertilizer plant: 28 years, no full inspection: Before 270 tons of ammonium nitratet exploded at ... http://t.co/XwUwgRcGDT \\ \cline{2-2} 
 &
  RT @mpoindc: I want them to know that they are not forgotten, Obama says to victims of explosion in West, TX. \\
 &
  I want them to know that they are not forgotten, Obama says to victims of explosion in West, TX. \\ \cline{2-2} 
 &
  RT @BreakingNews: Large explosion reported at fertilizer plant near Waco, Texas - @CBSDFW http://t.co/xOIyCyuxFD \\
 &
  Explosion reported at fertilizer plant near Waco, Texas - @CBSDFW http://t.co/xOIyCyuxFD \\ \cline{2-2} 
 &
  RT @BBCBreaking: 12 confirmed dead, approximately 200 injured in \#West fertilizer plant explosion in Texas, say state officials \\
 &
  Searchers Find 12 Bodies After Texas Explosion http://t.co/fnBc2LmXs (CNN) — Hundreds believed injured in Texas fertilizer plant explosion, medical examiner says. http://t ... \\ \cline{2-2} 
 &
  RT @laurenonizzle: This iPhone video of the fertilizer plant explosion near \#Waco will send chills up your spine. Surreal. http://t.co/O ... \\
 &
  RT @laurenonizzle: This iPhone video of the fertilizer plant explosion near \#Waco will send chills up your spine. Surreal. http://t.co/O ... \\ \cline{1-2} 
\multirow{10}{*}{SST-2 (100)} &
  smart , sassy interpretation of the oscar wilde play . \\
 &
  harp , sassy interpretation of the oscar wilde play , with an unexpected twist . \\ \cline{2-2} 
 &
  a fast paced and suspenseful argentinian thriller about the shadow side of play . \\
 &
  a fast paced and suspenseful argentinian thriller . \\ \cline{2-2} 
 &
  this comic gem is as delightful as it is derivative . \\
 &
  the film is bright and flashy in all the right ways . \\ \cline{2-2} 
 &
  the best movie in many a moon about the passions that sometimes fuel our best achievements and other times leave us stranded with nothing more than our lesser appetites . \\
 &
  the best film in many a moon about the passions that sometimes fuel our best achievements and other times leave us stranded with nothing more than our lesser appetites . \\ \cline{2-2} 
 &
  a fine production with splendid singing by angela gheorghiu , ruggero raimondi , and roberto alagna . \\
 &
  a fine production with splendid singing by angela gheorghiu , ruggero raimondi , and roberto alagna . \\ \cline{1-2} 
\end{tabularx}
\end{table*}

In our experiments, we also analyzed the generated data. For this we picked generated instances and tried to find the original instance, that has the closest resemblance (measured by Levenshtein distance). In Table \ref{table:generated_data} a excerpt of some instances, original and generated counterparts, from the West Texas Explosions and SST-2 datasets are given. Here we can see, that the GPT-2 model is, for example, able to remove preceding words (first and second instance of West Texas Explosions) or even truncate the sentence at the end (second instance of SST-2). The first example of the SST-2 dataset shows that the model is also able to enlarge the original instance. In case of the third example of West Texas Explosions it could be that the original instance is interpolated with another instance. The fourth instance of the SST-2 dataset also shows that the model can make small changes like synonym substitution. Furthermore, for many generated instances we were not able to find similar counterparts, see for example the third instance of the SST-2 dataset given in Table \ref{table:generated_data}. These can, for example, be instances the model learned beforehand, which supports the consideration that the model is able to create highly diverse examples with new linguistic features. However, as shown with the last examples of the two datasets, the model also sometimes repeats the original instance. In general, the findings indicate that the method proposed in our study is capable of performing many different transformations.
